# Supplementary material for: DAP: A Dynamic Adversarial Patch for Evading Person Detectors
Source: arXiv:2305.11618 source file (2023-11-20)
Supplement: Supplementary file 1 [file X_suppl.tex]

\clearpage
\setcounter{page}{1}
\maketitlesupplementary

%\section{Rationale}
%\label{sec:rationale}
% 
%Having the supplementary compiled together with the main paper means that:
% 
%\begin{itemize}
%\item The supplementary can back-reference sections of the main paper, for example, we can refer to \cref{sec:intro};
%\item The main paper can forward reference sub-sections within the supplementary explicitly (e.g. referring to a particular experiment); 
%\item When submitted to arXiv, the supplementary will already included at the end of the paper.
%\end{itemize}
% 
%To split the supplementary pages from the main paper, you can use \href{https://support.apple.com/en-ca/guide/preview/prvw11793/mac#:~:text=Delete%20a%20page%20from%20a,or%20choose%20Edit%20%3E%20Delete).}{Preview (on macOS)}, \href{https://www.adobe.com/acrobat/how-to/delete-pages-from-pdf.html#:~:text=Choose%20%E2%80%9CTools%E2%80%9D%20%3E%20%E2%80%9COrganize,or%20pages%20from%20the%20file.}{Adobe Acrobat} (on all OSs), as well as \href{https://superuser.com/questions/517986/is-it-possible-to-delete-some-pages-of-a-pdf-document}{command line tools}.

%=============================
\section{Limitations of GAN-based techniques}
%=============================
\begin{figure*}[ht]
\centering
\includegraphics[width=2\columnwidth]{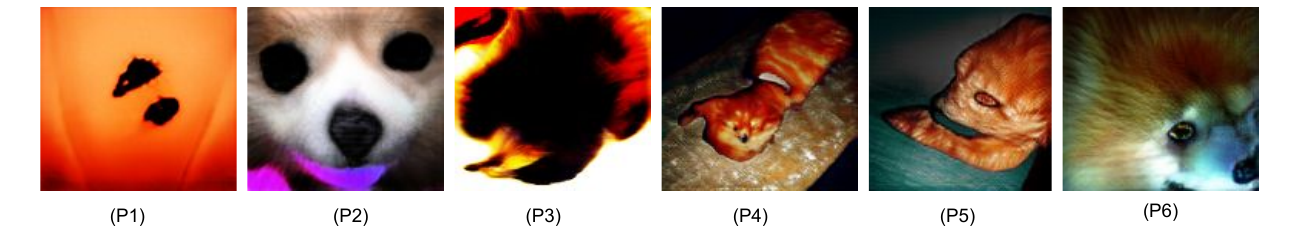}
\caption{Failed attempts to generate GAN-based naturalistic patches: (P1) on YOLOv3, (P2) on Faster-CNN, (P3), (P4), (P5), and (P6) on YOLOv2.}
\label{gan_2}
\end{figure*}
\noindent{\textbf{\textit{Limitation 1: Failure to converge}}}

%\begin{minipage}{\textwidth}
%\begin{minipage}[b]{0.4\textwidth}
%\centering
%\includegraphics[width=5.5cm,height=2cm]{figures/Gan_attempts_short.pdf}
%\captionof{figure}{\label{fig:gan}Failed attempts to generate GAN-based naturalistic patches: (P1) on YOLOv3, (P2) and (P3) on YOLOv2.}
%\end{minipage}
%\hfill
%\begin{minipage}[b]{0.58\textwidth}
%\centering
%\includegraphics[width=8cm,height=3cm]{figures/fail_attempt_conv.png}
%\captionof{figure}{\label{fig:gan_graph}Failed attempts to generate an efficient patch for different initialization.}
%\end{minipage}
%\end{minipage}

When attempting to reproduce the results of GAN-based approaches such as \cite{Hu21}, we found it to be inefficient, with the code failing to converge to realistic patterns in some cases. In the experiment, we generated patches for several datasets, including CASIA, wildtrack, and INRIA, using the BigGAN generator \cite{biggan} at an output resolution of $128 \times 128$, pre-trained on the ImageNet 1k dataset, with the class vector set to 'dog', as in \cite{Hu21}. The resulting patches, shown in Figure \ref{gan_2}, were trained on different object detectors, including YOLOv2, YOLOv3, and FasterCNN, with patch generation taking between 24 to 72 hours on a Geforce GTX 1080 ti, depending on the dataset size and the used pre-trained GAN. %Additionally, Figure \ref{fig:gan_graph} demonstrates that even when the generated patches had a naturalistic appearance, the success rate of the attack was minimal with different initializations.
%\textbf{Limitation 1:}
%Additional results are found in Figure \ref{gan_2}, the GAN-based technique failed to converge to realistic patterns.

%\textbf{Limitation 2:}
\noindent{\textbf{\textit{Limitation 2: Too limited latent space}}}\\
%We ran the same experiments while targeting the Yolov3tiny. First we compare the attack effectiveness for different combinations of transformations. We also tested different norm thresholds 
%\begin{figure*}[!ht]
%\includegraphics[width=2\columnwidth]{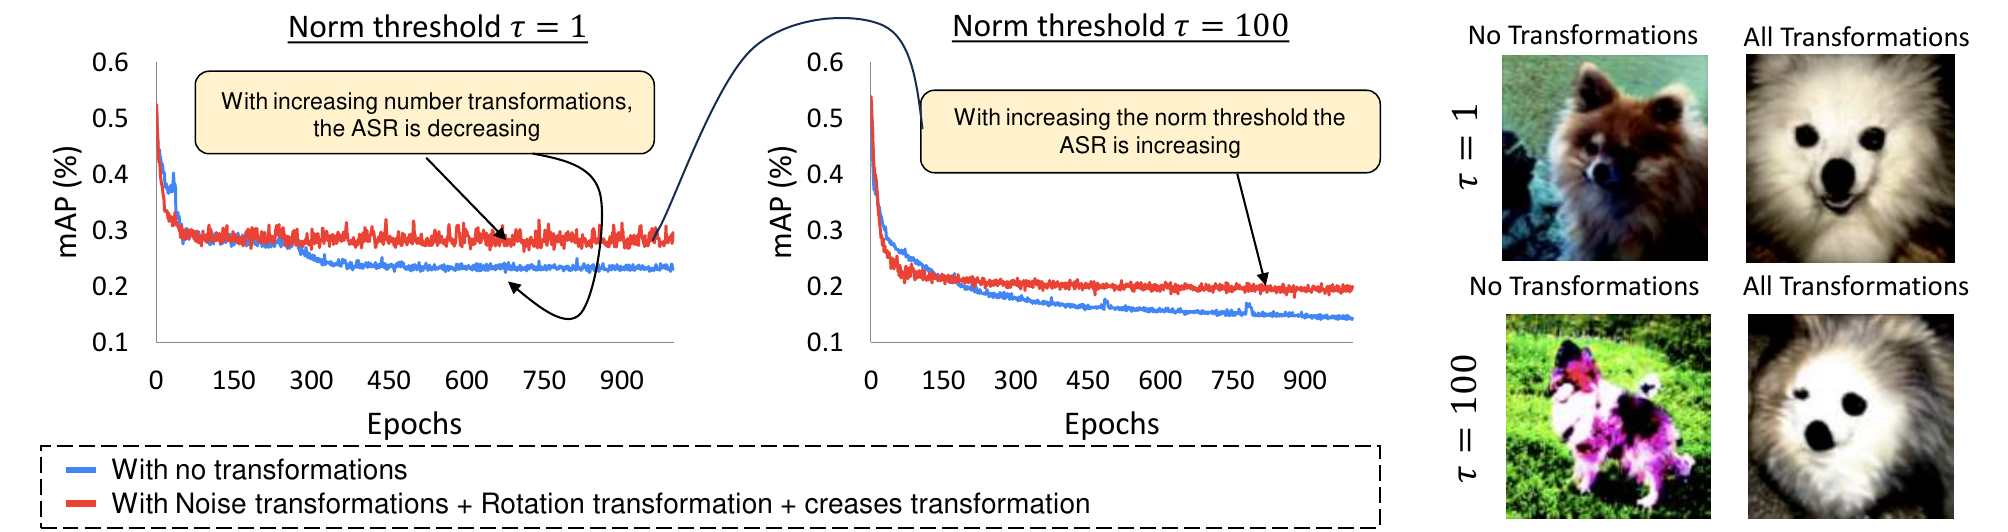}
%\caption{\label{Gan_performance_tiny}Mean Average Precision (mAP) convergence curves when training a GAN-based technique with and without different transformations. Illustrating the impact of adjusting the latent vector constraints on attack success rate (ASR) (\textit{Left:} $\tau = 1$ and \textit{Right:} $\tau = 100$) and the corresponding generated patch.}
%\end{figure*} 

\begin{figure*}[ht]
\includegraphics[width=\textwidth]{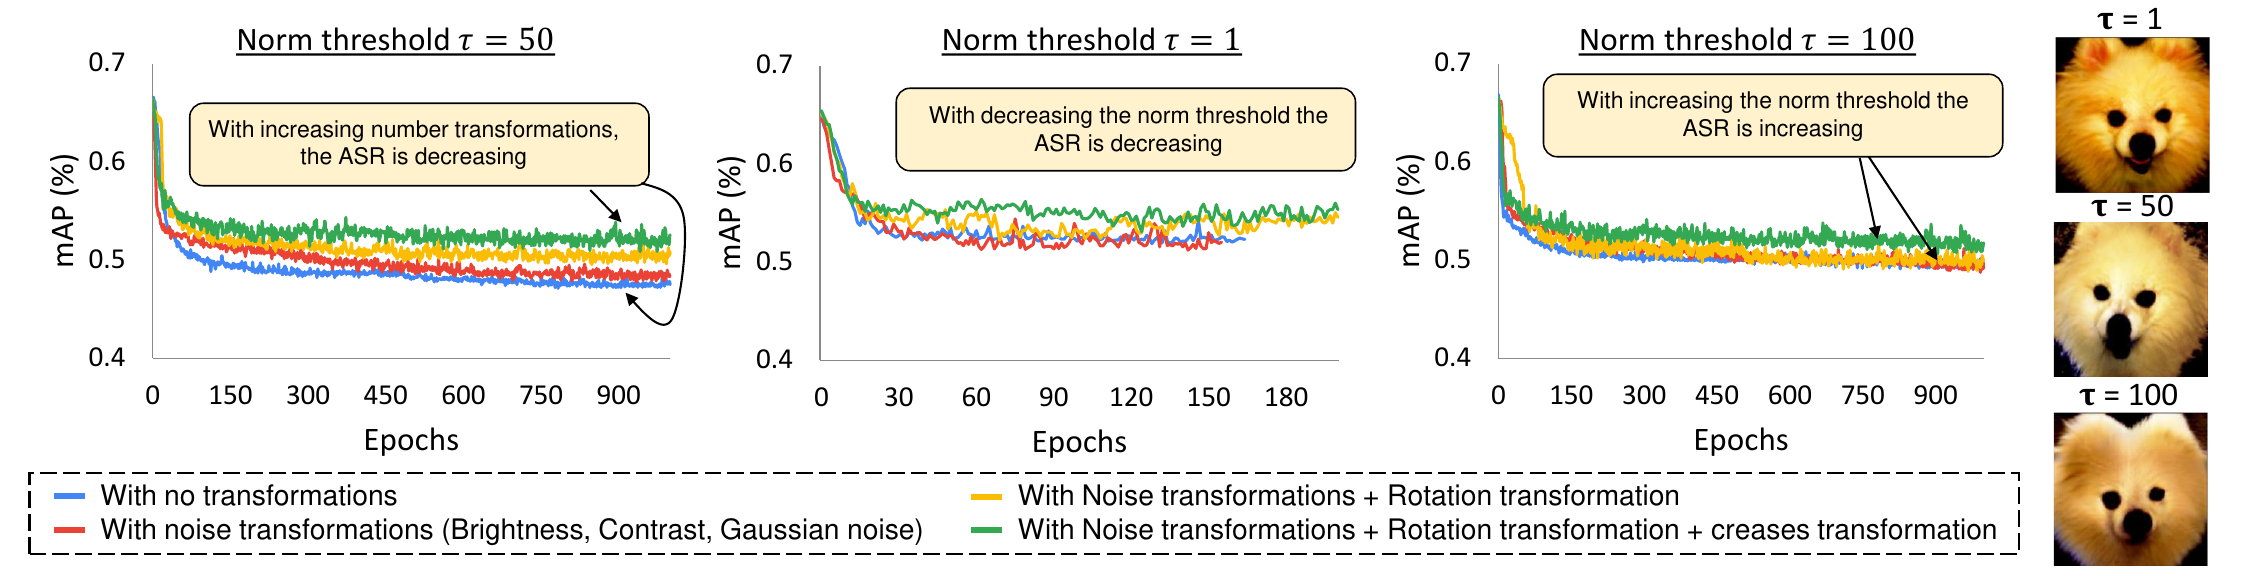}
\caption{\label{fig:transformation}Mean Average Precision (mAP) convergence curves when training a GAN-based technique with and without different transformations. Illustrating the impact of adjusting the latent vector constraints on attack success rate (ASR) (\textit{Left:} $\tau = 50$ (same used in \cite{Hu21}), \textit{Middle:} $\tau = 1$, and \textit{Right:} $\tau = 100$). Summary of these curves are presented in Table \ref{Gan_performance}}
\end{figure*} 

We run multiple experiments where we try to generate naturalistic patches with different combinations of transformations, i.e., without any transformations, with basic transformations (i.e. random noise, contrast and brightness variations), with basic transformations plus rotation, and when using all the transformations including the creases transformations that model wrinkles and creases in a person's cloth. Without loss of generality, we use the Yolov3 detector as our victim model.
As illustrated in Figure \ref{fig:transformation}-\textit{Left}, for a norm threshold $\tau=50$, the same value used in \cite{Hu21}, with the increase in the number of considered transformation the effectiveness of the attack decreases. This could be explained by the fact that the latent space of the GAN is too limited to find a patch that is robust to all the basic, rigid and non-rigid transformations at once. To illustrate this, we run experiments by adjusting the norm threshold of the latent vector (i.e., $\tau=1$ and $\tau=100$), and report the convergence of the mean average precision (mAP) of the generated patch while training. As shown in Figure \ref{fig:transformation}-\textit{Middle}, corresponding to a more strict constraint, i.e., $\tau=1$, the resultant patch converges to a higher mAP value leading to a lower attack success rate. We also test for $\tau=100$, we notice that the generated patches converge to a lower mAP compared to the $\tau=1$ case, which corresponds to a higher attack success rate. We present the final mAP for different experiments in Table \ref{Gan_performance}.
Figure \ref{fig:transformation} also shows the generated patches for different norm thresholds, where it can be noticed that the lower the threshold the more naturalistic the generated patch looks. To conclude, the norm threshold allows a trade-off between realism and attack efficiency.
%\noindent{\textbf{\textit{Limitation: Inefficiency when trained for multiple transformations}}}\\

\begin{table}[htp]
\centering
\small
  \begin{tabular}{lccc}
    \toprule
    \textbf{Transformations} & \textbf{$\tau = 1$}  & \textbf{$\tau = 50$} & \textbf{$\tau = 100$}   \\
    \midrule
      \textbf{No transformation}            &  52.81$\%$ & 47.57$\%$  &  49.67$\%$  \\
      \textbf{Noise}                        &  52.55$\%$ & 48.51$\%$  &  49.60$\%$ \\
      \textbf{Noise + Rotation}             & 54.05$\%$  & 50.44$\%$  & 49.99$\%$  \\
      \textbf{Noise + Rotation + Creases}   & 55.16$\%$  & 52.07$\%$  & 51.76$\%$ \\
  \bottomrule
\end{tabular}
\captionof{table}{\label{Gan_performance} mAP of GAN-based technique when training using different transformations.}
\end{table}
%=============================
\section{Impact of Patch Size}
%=============================
\begin{figure}[ht]
\centering
\includegraphics[width=0.8\columnwidth]{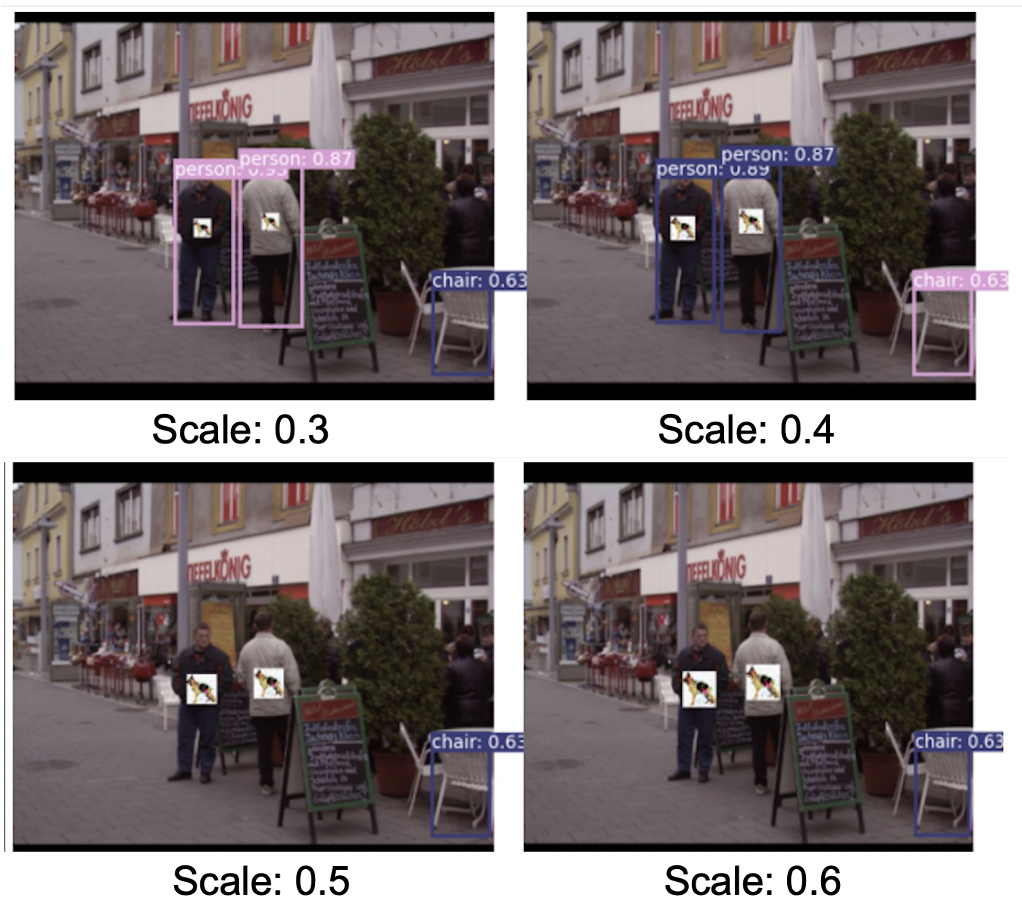}
\captionof{figure}{\label{Fig:size}Illustration of different patch scales.}
\end{figure}

To assess the impact of patch size on the efficacy of our proposed adversarial patch, a series of digital experiments were carried out on the INRIA dataset. The objective was to evaluate how different patch sizes affect the effectiveness of our approach. Figure \ref{Fig:size} visually represents the various scales employed to generate distinct patches on the targeted objects. It is worth noting that a scale of 0.5 in our experiments corresponds to a scale of 0.2 as described in \cite{Hu21}. By conducting these experiments and analyzing the outcomes, we aimed to gain insights into the relationship between patch size and the performance of our adversarial patch, ultimately providing valuable information for optimizing its effectiveness.

%=============================
\section{Cross-Dataset Evaluation}
%=============================
\begin{table}[htp]
\small
\centering
  \begin{tabular}{lc}
    \toprule
    \textbf{Datasets} & \textbf{mAP}\\
    \midrule
      \textbf{INRIA}  & 15.44$\%$     \\
      \textbf{MPII}  &  19.32 $\%$   \\
 \bottomrule
  \end{tabular}
  \caption{\label{performance-cross}Attack performance (mAP) of DAP on MPII.}
\end{table}
We employed Yolov3tiny for training an adversarial patch using the INRIA dataset, and subsequently evaluated the performance of the generated patch on the MPII dataset \cite{MPII}. Table \ref{performance-cross} presents the results of this cross-dataset testing. Remarkably, our adversarial patch exhibited impressive transferability between datasets. Specifically, a patch generated using the INRIA dataset, with a mean average precision (mAP) of $15.44\%$, demonstrated a notable effectiveness on the MPII dataset, achieving a mean precision accuracy (mPA) of $19.32\%$. This significant finding underscores the robustness and generalizability of our approach. It indicates that an adversarial patch tailored to one dataset can still exhibit strong performance and yield desirable outcomes when applied to a different dataset, such as MPII.

%=============================

\begin{figure}[!ht]  %{l}{5cm}
\centering
\includegraphics[width=\columnwidth]{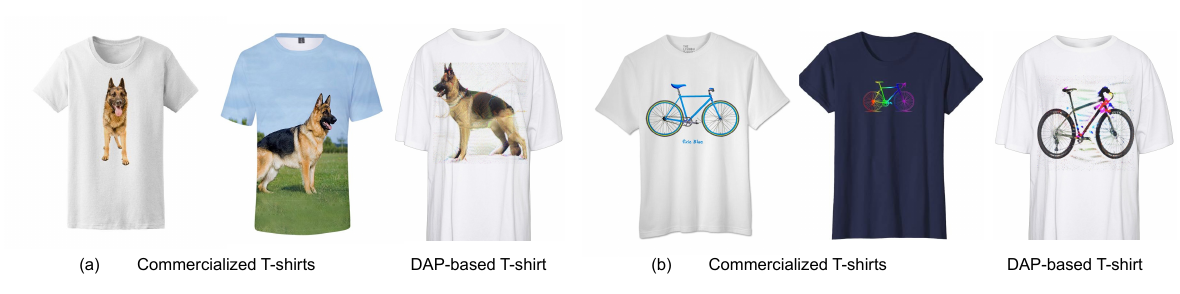}
\caption{DAP-based T-shirts vs Commercialized T-shirts: (a) Dog-based, (b) Bicycle-based. Our DAP-based T-shirt seems indistinguishable from other commercialized T-shirts.}\label{DAP_vs_commercial}
\end{figure}

%=============================
\section{Performance of our Attack: Physical World Experiments}
To evaluate the real-world effectiveness of our proposed adversarial patch, we conducted a physical attack experiment where we printed the patch and tested its performance in a real-world setting. %Specifically, we used the YOLOv3tiny-based adversarial patch shown in Figure \ref{result_1}. 
In the experiment, we took pictures of one person holding the printed patch and tested whether it could successfully evade detection by an object detector. For the with deformations setting, we added random creases to the paper by crumpling this latter. 
The results of this experiment are illustrated in Figure \ref{with_wrinkles_phys} (additional real-world evaluation results are provided in the supplementary materials). 
%\textcolor{red}{we need numerical results}
\begin{table}[!ht]
  \small
    \centering
    \begin{tabular}{cccc}
    \toprule
        \textbf{} & \textbf{Benign} & \textbf{NAP} & \textbf{DAP} \\
        \midrule
         Without creases &  100\%   &  30\% & 75\%\\
         With creases &  100\%   &  20\% & 65\%\\
    \bottomrule
    \end{tabular}    
    \caption{Attack Success Rate (ASR) in Benign scenarios and when using DAP and NAP \cite{Hu21} when attacking Yolov3tiny with and without creases.}
    \label{tab:detection_CT}
\end{table}

We carried out our real-world experiments using a set of 100 test samples, each featuring a person holding a printed patch. These samples encompassed a range of transformations, such as rotation, resizing, perspective changes, and other variations.
Moreover, we report the attack success rate as an indicator of the effectiveness of our approach in the context of these real-world transformations.
Our proposed patch maintained its effectiveness for different distances from the camera, different angles, different scales and for different lighting conditions. Table \ref{tab:detection_CT} reports the patch success rate in the physical world and when using our DAP, only 35\% of the time a person is detected.

\begin{figure}[!ht]
\centering %width=8cm,height=2.5cm
\includegraphics[width=\columnwidth]{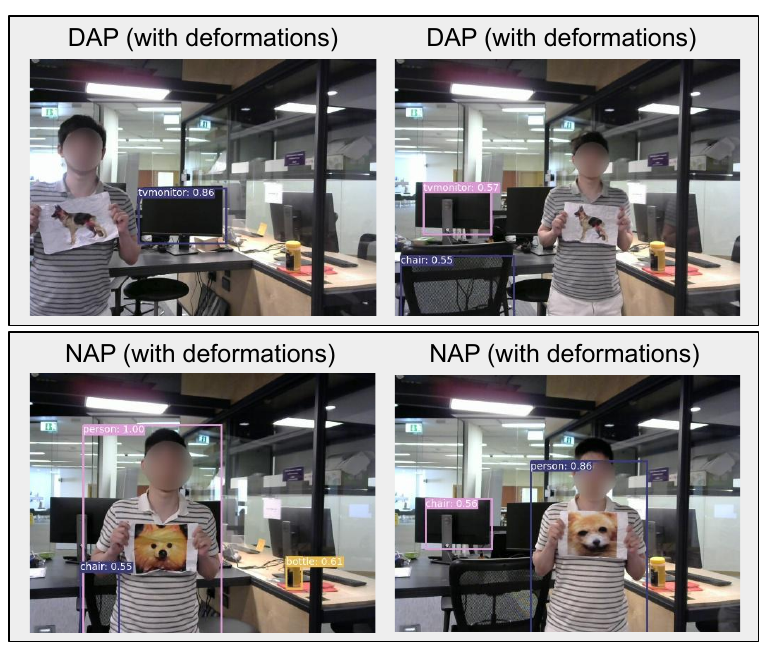}
\caption{Detection results when applying random creases and rotations to the DAP patches (\textit{upper}) for Yolov3tiny and NAP patches (\textit{lower}) for Yolov3 and Yolov3tiny.}\label{with_wrinkles_phys}
\end{figure}
As shown in Figure \ref{with_wrinkles_phys}, even after being rotated, our patch was still effective in hiding the person from detection. In contrast, when we applied the same deformations to the naturalistic patches from \cite{Hu21} (NAP), we found that the patch was no longer effective in evading detection. This highlights the strength of our proposed patch, which is more robust to physical deformations and can maintain its effectiveness even when the patch is crumpled and rotated. As shown in Table \ref{tab:detection_CT}, the detection recall dropped to 45\% even with the presence of multiple creases in the patch in addition to applying rotations.

%\begin{table}[!ht]
%  \small
%    \centering
%    \begin{tabular}{cccc}
%    \toprule
%        \textbf{} & \textbf{Without patch} & \textbf{NAP} & \textbf{DAP} \\
%        \midrule
%         Attack Success Rate (ASR) &  100\%   &  20\% & 65\%\\
%    \bottomrule
%    \end{tabular}    
%    \caption{Attack Success Rate (ASR) of DAP and NAP \cite{Hu21} when using Yolov3tiny with wrinkles.}
%    \label{tab:detection_with_CT}
%\end{table}
%=============================
\section{Real World Experiments}
%=============================
To thoroughly evaluate the robustness of our adversarial patch, we subjected the T-shirt, along with our patch, to aggressive transformations. Notably, even under these challenging conditions, our patch consistently outperformed the GAN based patch. Despite the aggressive transformations applied to the T-shirt, our patch demonstrated remarkable resilience and maintained its effectiveness in evading detection (See Figure \ref{deformation_dap}). In contrast, the NAP patch struggled to retain its deceptive properties under similar transformations (See Figure \ref{deformation_gan}). These findings provide compelling evidence of the superior performance and robustness of our adversarial patch in the face of extreme alterations. Our patch's ability to withstand aggressive transformations further underscores its potential for reliable and effective evasion of detection systems, solidifying its superiority over the GAN-based patch.

\begin{figure*}[!ht]
\centering
\includegraphics[width=2\columnwidth]{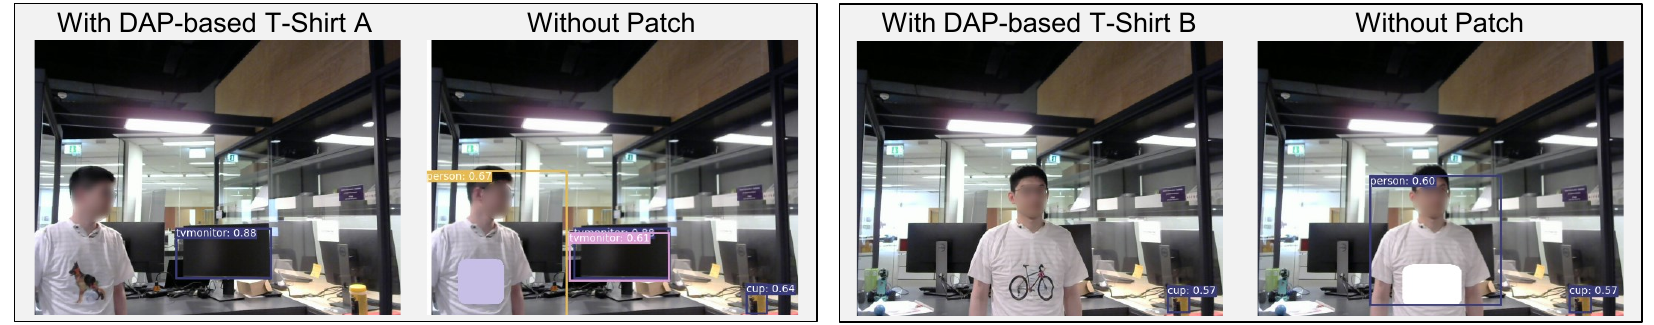}
\caption{Detection results of with and without our DAP-based T-shirt for other classes.}
\label{result_4}
\end{figure*}

\begin{figure*}[!ht]  %{l}{5cm}
\centering
\includegraphics[width=2\columnwidth]{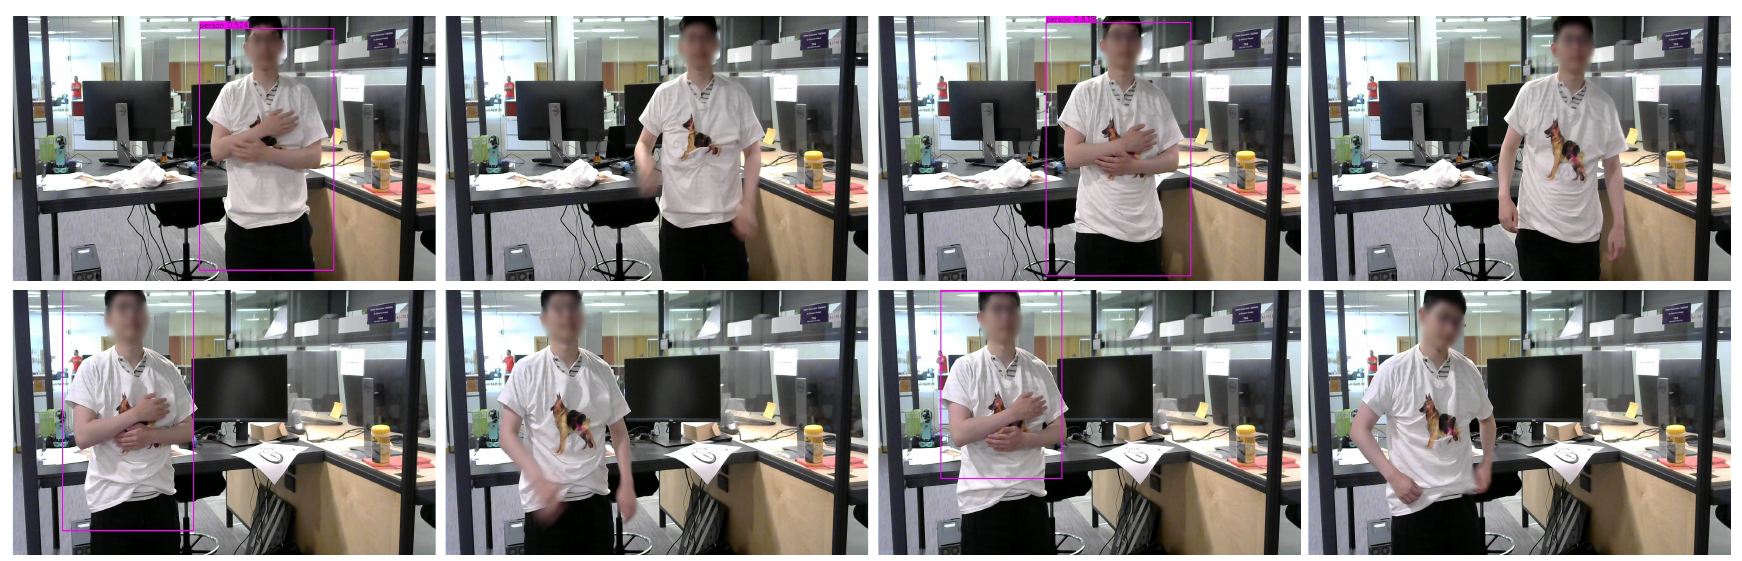}
\caption{DAP-based T-shirts performance while applying different deformations.}\label{deformation_dap}
\end{figure*}

\begin{figure*}[!ht]  %{l}{5cm}
\centering
\includegraphics[width=2\columnwidth]{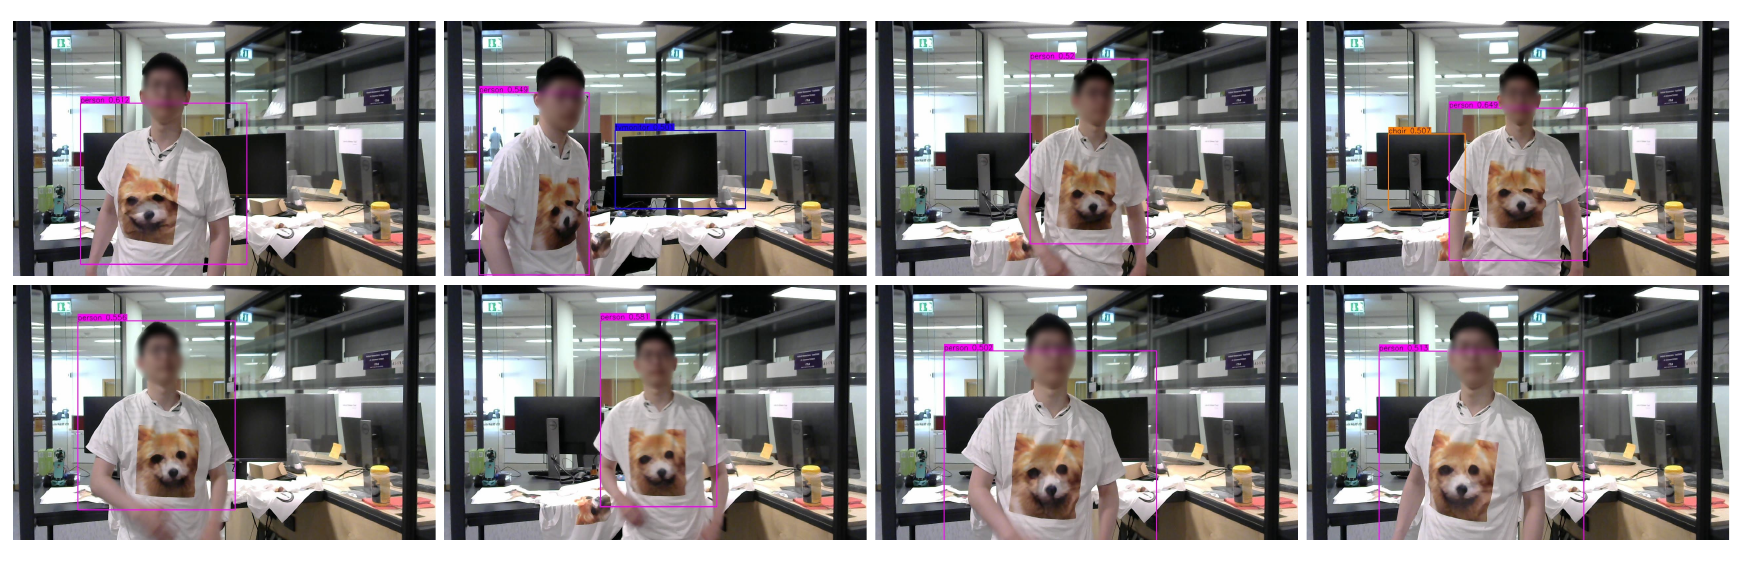}
\caption{NAP-based T-shirts performance while applying different deformations.}\label{deformation_gan}
\end{figure*}

To illustrate this annotation process, Figure \ref{annotation} showcases four different cases. The key metrics used to evaluate the performance of the detection system are as follows:

\begin{itemize}
    \item True Positive Rate (TPR): This represents the percentage of total results that are correctly identified as positive, specifically when a patch is present and the person is not detected ($P=1~ \& ~D=0$). It is computed as: ${\displaystyle \mathrm {TPR} ={\frac {\mathrm {TP} }{\mathrm {P} }}={\frac {\mathrm {TP} }{\mathrm {TP} +\mathrm {FN} }} }$.
    \item False Positive Rate (FPR): This indicates the percentage of total test results that are incorrectly identified as positive, occurring when a patch is present and a person is detected ($P=1~ \& ~D=1$). It is calculated as: ${\displaystyle \mathrm {FPR} ={\frac {\mathrm {FP} }{\mathrm {N} }}={\frac {\mathrm {FP} }{\mathrm {FP} +\mathrm {TN} }} }$.
    \item True Negative Rate (TNR): This corresponds to the percentage of cases ($P=0~ \& ~D=1$) where the patch is not present, and the person is correctly detected. It is calculated as: ${\displaystyle \mathrm {TNR} ={\frac {\mathrm {TN} }{\mathrm {N} }}={\frac {\mathrm {TN} }{\mathrm {TN} +\mathrm {FP} }} }$.
    \item False Negative Rate (FNR): This represents the percentage of cases where the detector fails to detect a person even though the patch is not present ($P=0~ \& ~D=0$). It is calculated as: ${\displaystyle \mathrm {FNR} ={\frac {\mathrm {FN} }{\mathrm {P} }}={\frac {\mathrm {FN} }{\mathrm {FN} +\mathrm {TP} }} }$.
\end{itemize}
These evaluation metrics allow us to assess the performance of our adversarial patches and provide quantitative insights into the detection results obtained during our experiments.

%\begin{figure}[ht]
%\centering
%\includegraphics[width=\columnwidth]%{figures/results_detectors_2_blurred.pdf}
%\caption{Detection results for different detectors, angles, distances from the camera, scales, and lighting conditions.}
%\label{result__}
%\end{figure}

%=============================
\section{Adversarial Patches in Different Classes}
%=============================
%\begin{wrapfigure}{l}{7cm}
%  \includegraphics[width=7cm,height=3cm]{figures/other_classes_2_blurred.pdf}
%\captionof{figure}{\label{other_classes}Detection results with different classes.}
%\end{wrapfigure}

In addition to our digital experiments, we conducted physical world experiments to further validate the effectiveness of our approach. In these experiments, we selected alternative target natural images, such as Bicycles and Cats, and tested the performance of the generated adversarial patches. To ensure practical applicability, the patches were printed on A4 papers. Figure \ref{result_cat_bicycle} provides a visual representation of our findings. Across various scales, rotation angles, lighting conditions, and distances from the camera, our proposed patches consistently exhibited high efficacy in concealing the presence of a person and deceiving the detector. These physical world experiments serve as compelling evidence of the real-world viability and robustness of our adversarial patch methodology, further supporting its potential for practical implementation and deployment.

\begin{figure*}[ht]
\centering
\includegraphics[width=2\columnwidth]{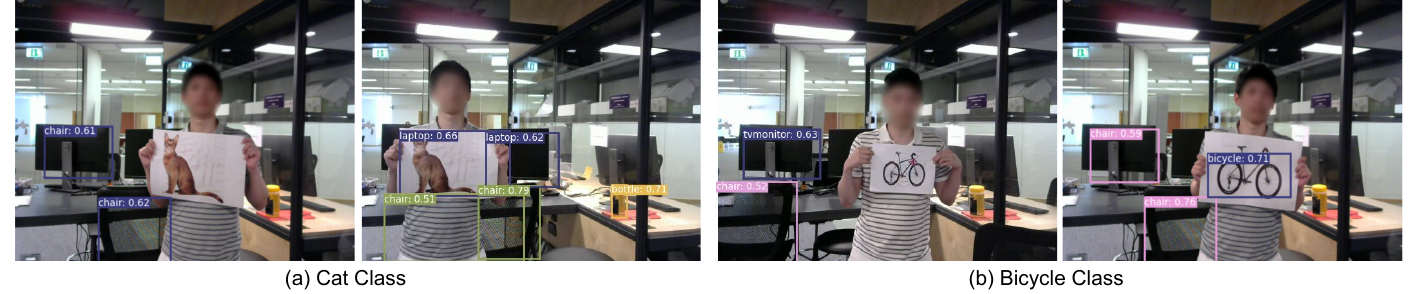}
\caption{Detection results for different angles, distances from the camera, scales, and lighting conditions for Cat and Bicycle-based DAP.}
\label{result_cat_bicycle}
\end{figure*}

In our pursuit of assessing the real-world applicability of our approach, we went a step further and introduced creases to the adversarial patches targeting specific classes, such as the bicycle class. By crumpling the paper containing the patch, we aimed to simulate real-world scenarios that could potentially impact the patch's effectiveness. Figure \ref{result_2} visually demonstrates the outcomes of these experiments. Despite the introduction of creases and the resultant deformation of the patch, we observed that its effectiveness remained intact. The patch continued to effectively hide the targeted object. %, reinforcing the resilience of our proposed method even in challenging physical conditions.
%These experiments demonstrate the robustness of our adversarial patch against environmental factors and physical alterations, underscoring its potential for reliable performance in real-world scenarios.

\begin{figure}[ht]
\centering
\includegraphics[width=\columnwidth, height = 3cm]{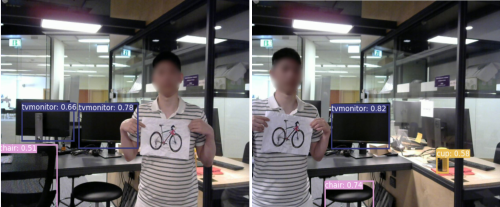}
\caption{Detection results when adding creases to the Bicycle class-based DAP.}
\label{result_2}
\end{figure}

\begin{figure}[!ht]
\centering
\includegraphics[width=\columnwidth]{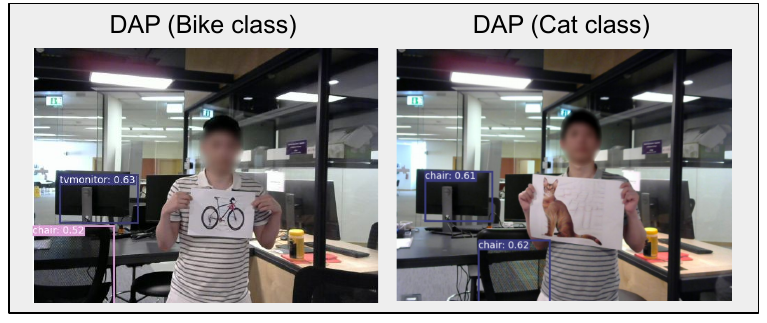}
\caption{Detection results for other classes.}
\label{result_3}
\end{figure}

%------------------------------------------
%\subsubsection{Impact of Adding Creases on Other Classes based Patch}
%------------------------------------------

%------------------------------------------
\section{Patch robustness against Input Transformation-based Defenses}
%------------------------------------------

To further evaluate the robustness of our proposed adversarial patch, we tested it against three commonly used defense approaches that perform input transformations without re-training the victim models. Specifically, we applied JPEG compression \cite{jpeg}, added Gaussian noise \cite{gaussian}, and applied Median blurring \cite{median} to the input images. To assess the effectiveness of our patch under these defense techniques, we measured the mean average precision of both the benign and adversarial scenarios. Our experimental results, presented in Table \ref{defense}, demonstrate that our proposed patch remains effective even when these defense techniques are applied to the input images. These findings suggest that our proposed patch has the potential to be effective in real-world scenarios where defense mechanisms are commonly employed to protect against adversarial attacks. Further research can explore the development of more robust defense techniques, as well as more advanced and sophisticated adversarial patches.

 \begin{table*}[!ht]
  \centering
\small
  \begin{tabular}{ccccccccc}
   \toprule
    \multicolumn{3}{c}{\textbf{JPEG}}&  \multicolumn{3}{c}{\textbf{Median Blurring}}&  \multicolumn{3}{c}{\textbf{Gaussian Noise}}\\
    \cmidrule(r){1-3} \cmidrule(r){4-6} \cmidrule(r){7-9}
    \textbf{Param} & \textbf{Benign }& \textbf{Adv}&\textbf{Param} & \textbf{Benign }& \textbf{Adv}& \textbf{Param} &\textbf{Benign }& \textbf{Adv}\\
    \midrule
      \textbf{90}  &   98.03$\%$   & 25.34$\%$  & \textbf{5}  &   99.3$\%$   & 22.34$\%$  & \textbf{0.01}  &   80$\%$   & 45.3$\%$ \\
      \textbf{70}  &   95.3$\%$  & 31.98$\%$  & \textbf{10}  &   96.76$\%$  & 21.12$\%$ & \textbf{0.02}  &   75.1$\%$  & 47.43$\%$\\
      \textbf{50}  &   90.23$\%$  & 42$\%$ & \textbf{15}  &   93.44$\%$  & 42.2$\%$ & \textbf{0.05}  &   78.65$\%$  & 50.2$\%$\\
     \textbf{30}  &   80.1$\%$  & 50.5$\%$ & \textbf{20}  &   87.30$\%$  & 30.11$\%$ &  \textbf{0.1}  &   70.44$\%$  & 55.23$\%$\\
  \bottomrule
\end{tabular}
  \caption{\label{defense} Attack performance of adversarial patch when using JPEG Compression, Median Blurring, and Gaussian Noise defense in a benign and adversarial scenarios for different defense parameters.}
\end{table*}
